# Supplementary material for: Learning-Based Approaches to Predictive Monitoring with Conformal Statistical Guarantees
Source: arXiv:2312.01959 source file (2023-12-04)
Supplement: Supplementary file 1 [file appendix.tex]

\appendix

\section{Bayesian Inference}\label{app:bayes}

\subsubsection{Gaussian Processes} Gaussian Processes (GP) are a well-known formalism to define distributions over real-valued functions of the form $g: X\to \mathbb{R}$. A GP distribution is uniquely identified by its mean $\mu(x)=\mathbb{E}[g(x)]$ and its covariance function $k_\gamma(x,x')$ and characterized by the fact that the distribution of $g$ over any finite set of points $\hat{x}$ is {Gaussian} with mean $\mu(\hat{x})$ and variance $k_\gamma(\hat{x},\hat{x})$.  
In the following, we let $g_t$, $\mu_t$ and $K_{N_tN_t}$ denote respectively the latent, the mean and the covariance functions evaluated on the training inputs $X_t$.

The GP prior over latent functions $g$ evaluated at training inputs $X_t$ -- step 1 -- is defined as $p(g|X_t) = \mathcal{N}(g|\mu_t, K_{N_tN_t})$. The posterior over latent variables $p(g_t|Z')$ -- step 3 -- is not available in closed form since it is the convolution of a Gaussian and a binomial distribution. 
Hence, we have to rely on SVI for  posterior approximation (details later).  Once we obtain a tractable posterior approximation, in order to make predictions over a test input $x_*$, with latent variable $g_*$, if we want to restrict the output space from $\mathbb{R}$ to $[0,1]$ (e.g. in classification problems) we need to compute an empirical approximation of the predictive distribution
\begin{equation}\label{eq:pred_gp}
    p(f_*|x_*,Z') = \int \Phi (g_*)p(g_*|x_*, Z')dg_*,
\end{equation}
in which the outputs of the latent function $g:\Theta\to \mathbb{R}$ are mapped into the $[0, 1]$ interval by means of a so-called link function $\Phi$, typically the inverse logit or the inverse probit function~\cite{bishop2006pattern}, so that $f:\Theta\to [0,1]$ is obtained as $f = g \circ \Phi$.

\paragraph{Stochastic Variational Inference.}
Here we outline an intuitive explanation of the SVI steps to approximate the GP posterior when the likelihood is non-Gaussian. 
The main issue with GP inference is the inversion of the $N_t\times N_t$ covariance matrix $K_{N_tN_t}$. This is the reason why variational approaches to GP start with sparsification, i.e. with the selection of $m \ll N_t$ inducing points that live in the same space of $X_t$ and, from them, define a set of inducing variables $u_t$. The covariance matrix over inducing points, $K_{mm}$, is less expensive to invert and thus it acts as a low-rank approximation of $K_{N_tN_t}$. We introduce a Gaussian variational distribution $q(u_t)$ over inducing variables whose goal is to be as similar as possible to the posterior $p(u_t|Z')$. A classical VI result is to transform the expression of the KL divergence between the variational distribution $q(u_t)$ and the posterior $p(u_t|Z')$ into a lower bound over the marginal log-likelihood $\log p(Z')$. As our
likelihood -- step 2 -- factors as $p(Z' | g_t ) = \prod_{i=1}^{N_t} p(L_i | g_i )$ and because of the Jensen inequality we obtain the following ELBO:

\begin{equation}\label{eq:gp_svi_bound}
   \log p(Z')\ge \sum_{i=1}^{N_t}\mathbb{E}_{q(g_i)}[\log p(L_i|g_i)]-KL[q(u_t)||p(u_t)]:= \mathcal{L}_{GP}(\nu,  \gamma),
\end{equation}
where $L_i$ denotes the set of observed Boolean tuples corresponding to points in $xi$ in $Z'$, $p(u_t)$ denotes the prior distribution over inducing variables and $\nu$ denotes the hyper-parameters introduced to describe the sparsification and the variational distribution. The distribution $q(g_t)$ is Gaussian with an exact analytic derivation from $q(u_t)$ that requires $\mathcal{O}(m^2)$ computations.
The SVI algorithm then consists of maximizing $\mathcal{L}_{GP}$ with respect to its parameters using gradient-based stochastic optimization. We stress that, at this step, the selection of inducing variable is optimized, resulting in a more effective sparsification. Computing the KL divergence in~\eqref{eq:gp_svi_bound} requires only $\mathcal{O}(m^3)$ computations. Most of the work will thus be in computing the
expected likelihood terms. 
Given the ease of parallelizing
the simple sum over $N_t$, we can optimize $\mathcal{L}_{GP}$ in a stochastic fashion by selecting mini-batches of the data at random.

\paragraph{Predictive distribution.} The predictive posterior $p(g_*|x_*, Z')$ is now approximated by a variational distribution $q(g_*)$, which is Gaussian and whose mean and variance can be analytically computed with cost $\mathcal{O}(m^2)$. From the mean and the variance of $q(g_*)$, we obtain the respective credible interval and we can use the link function $\Phi$ to map it to a subset of the interval $[0,1]$, in order to obtain the mean and the credible interval of the posterior predictive distribution $p(f_*|x_*, Z')$ of equation~\eqref{eq:pred_gp}.

\subsubsection{Bayesian Neural Networks}\label{sec: bnn}
The core idea of Bayesian neural networks (BNNs)~\cite{gal2016uncertainty,lampinen2001bayesian,titterington2004bayesian,goan2020bayesian,bishop2006pattern}, is to place a
probability distribution over the weights $\mathbf{w}$ of a neural network $f_{\mathbf{w}}:X\to T$, transforming the latter into a probabilistic model.
The inference process starts by defining a prior distribution $p(\mathbf{w})$ over $\mathbf{w}$ -- step 1 -- that expresses our initial belief about the values of the weights. 
As we observe data $Z'$, we update this prior to a posterior distribution $p(\mathbf{w}|Z')$ -- step 3 -- using Bayes' rule.

Because of the non-linearity introduced by the
neural network function $f_{\mathbf{w}}(x)$ and since the likelihood $p(Z'|\mathbf{w})$ -- step 2 -- may be non-Gaussian, the posterior $p(\mathbf{w}|Z')$ is non-Gaussian and it cannot be computed analytically. 
In order to predict the satisfaction function over an unobserved input $x_*$, we marginalize
the predictions with respect to the posterior distribution
of the parameters, obtaining 
\begin{equation}\label{eq:bnn_predictive}
    p(f_*|x_*, Z') = \int f_\mathbf{w}(x_*) p(\mathbf{w}|Z')d\mathbf{w}.
\end{equation}
The latter is called \emph{posterior predictive} distribution and it can be used to retrieve information about the uncertainty of a specific prediction $f_*$.
Unfortunately, the integration is analytically intractable due to the non-linearity of the neural network function~\cite{bishop2006pattern,mackay1992practical} so we empirically estimate such quantity.

Since precise inference is infeasible, various approximate methods have been proposed to infer a BNN. We consider two approximate solution methods: Stochastic Variational Inference and Hamiltonian Monte Carlo. 

\paragraph{Stochastic Variational Inference.}
 The rationale of SVI for BNNs is to choose a parametric variational distribution $q_\psi(\mathbf{w})$ that approximates the unknown posterior distribution $p(\mathbf{w}|Z')$ by minimizing the KL divergence $KL[q_\psi(\mathbf{w})||p(\mathbf{w}|Z')]$ between these two distributions. Since the posterior distribution is not known, the classic variational approach is to transform the minimization of the KL divergence into the maximization of the Evidence Lower Bound (ELBO)~\cite{jordan1999introduction}, defined as
\begin{equation}\label{eq:elbo}
    \mathcal{L}_{BNN}(\psi) := \mathbb{E}_{q_\psi(\mathbf{w})}\left[\log p(Z'|\mathbf{w})\right]-KL\left[q_\psi(\mathbf{w})||p(\mathbf{w})\right]\le \log p(Z').
\end{equation}
The first term is the expected log-likelihood of our data with respect to values of $f_\mathbf{w}$ sampled from $q_\psi(\mathbf{w}|Z')$, whereas the second term is the KL divergence between the proposal distribution and the prior. The distribution $q_\psi$ should be a distribution easy to sample from and such that the KL divergence is easy to compute. A common choice for $q_\psi$ is the Gaussian distribution (where $\psi$ denotes its mean and variance). KL divergence among two Gaussian distributions has an exact analytical form, hence the ELBO of~\eqref{eq:elbo} can be computed and it can be used as the objective function of a maximization problem over $\psi$.

\paragraph{Hamiltonian Monte Carlo.} (HMC)~\cite{neal2011mcmc}
defines a Markov chain whose invariant distribution is exactly the posterior $p(\mathbf{w}|Z')$ .
The Hamiltionian dynamics is used to speed up the space exploration. HMC does not make any assumption on the form of the posterior distribution, and is asymptotically correct. 
After convergence, HMC returns a trace of 
explored network weights $w_0, w_1, \ldots, w_N$
that, all together, can be interpreted as an empirical approximation of the posterior $p(\mathbf{w}|Z')$. Controlling in a precise way the convergence rate and how well the chain explores the parameter space is, however, far from trivial.

\paragraph{Predictive distribution.} The predictive distribution~\eqref{eq:bnn_predictive} is a non-linear combination of Gaussian distributions, and thus it is not Gaussian. However, samples can be easily extracted from its approximation, which allows us to obtain an empirical approximation of the predictive distribution. Let $\it [w_1,\dots, w_C]$ denote a vector of $C$ realizations of the random variable. Each realization $w_i$ induces a deterministic function $f_{w_i}$ that can be evaluated at $x_*$, the unobserved input, providing an empirical approximation of $p(f_*|x_*, Z')$.
